# Supplementary material for: Reconfigurable Intelligent Surfaces Enhanced NOMA D2D Communications Underlaying UAV Networks
Source: arXiv:2307.16086 source file (2023-08-01)

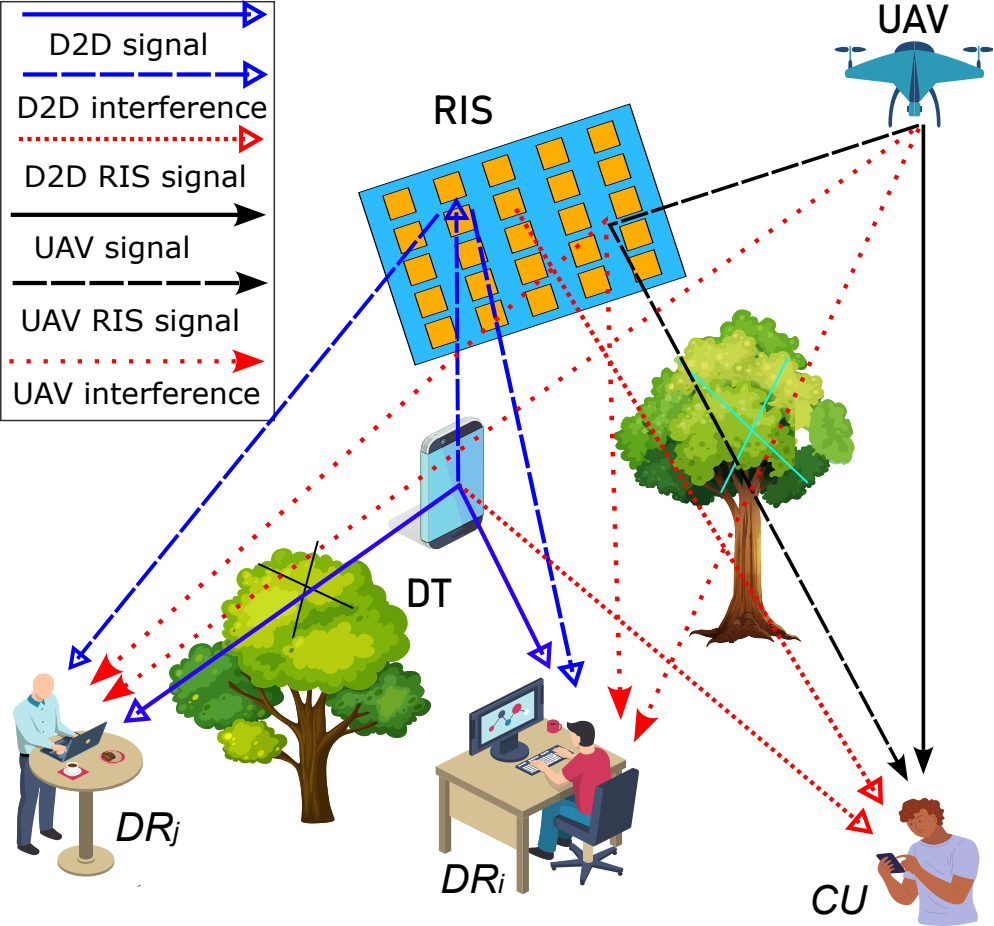

Supplement: Supplementary file 1 [file SM1.pdf]
